# Supplementary material for: Enhancing Photon Correlations through Plasmonic Strong Coupling
Source: arXiv:1701.08964 ancillary file (2017-10-06)
Supplement: Supplementary file 1 [file photon_statistics_SM.pdf]

# Enhancing Photon Correlations through Plasmonic Strong Coupling: Supplemental Material

R. Sáez-Blázquez,[1] J. Feist,[1] A. I. Fernández-Domínguez,[1,*] and F. J. García-Vidal[1,2,†]

[1]*Departamento de Física Teórica de la Materia Condensada and Condensed Matter Physics Center (IFIMAC), Universidad Autónoma de Madrid, E- 28049 Madrid, Spain*

[2]*Donostia International Physics Center (DIPC), E-20018 Donostia/San Sebastián, Spain*

This Supplemental Material provides details on different aspects of the theory presented in the main text. In Section 1, the effective Hamiltonian approach in the low pumping (perturbative) regime is tested against full Liouvillian calculations. Section 2 analyzes the impact that spatial inhomogeneities in the plasmon (SP) near-field have on far-field intensity and correlations. Spectral inhomogeneous broadening in the quantum emitter (QE) ensemble is investigated in Section 3. The effect of SP losses and QE non-radiative decay on the second-order correlation function of plasmon-exciton-polariton (PEP) systems is studied in Section 4. Finally, Section 5 explores the sensitivity of photon correlations against dipole-dipole interactions within the emitter ensemble. All the calculations presented correspond to hybrid systems involving five QEs ($\boldsymbol{N}=\mathbf{5}$).

## EFFECTIVE HAMILTONIAN VERSUS FULL LIOUVILLIAN

As discussed in the main text, the effective non-Hermitian Hamiltonian [1], $\hat{H}_{\rm eff}$ in Equation (3), is obtained by taking the low pumping limit in the full steady-state Liouvillian in Equation (1). The refilling terms in the Lindblad super-operators describing SP and QE radiative and nonradiative damping can be neglected in this limit. These ensure the normalization of the steady-state density matrix, $\hat{\rho}$. This condition can be relaxed in the low pumping regime, in which the population concentrates at the ground state $|0\rangle$ (no excitations in the system). Thus, we can set $\mathrm{Tr}\{\hat{\rho}\}\simeq\langle 0|0\rangle=1$, and approximate the Lindblad super-operators by

$$\mathcal{L}_{\hat{a}}[\hat{\rho}]\simeq-\{\hat{a}^\dagger\hat{a},\hat{\rho}\},\tag{1}$$

$$\mathcal{L}_{\hat{S}^-}[\hat{\rho}]\simeq-\{\hat{S}^+\hat{S}^-,\hat{\rho}\},\tag{2}$$

$$\sum_{i=1}^{N}\mathcal{L}_{\hat{\sigma}_i}[\hat{\rho}]\simeq-\{\sum_{i=1}^{N}\hat{\sigma}_i^\dagger\hat{\sigma}_i,\hat{\rho}\}=-\{\hat{S}_z,\hat{\rho}\}.\tag{3}$$

This not only allows describing the steady-state of the system in terms of an effective Hamiltonian, but more importantly, it also removes its dependence on the dark states of the QE ensemble, see Equations 2-3.

We can take further advantage of the low pumping limit inherent to $\hat{H}_{\rm eff}$ by treating it perturbatively on the incident laser amplitude, $E_{\rm L}$ [2]. This way, we can write $\hat{H}_{\rm eff}=\hat{H}_0+E_{\rm L}\hat{V}$ with

$$E_{\rm L}\hat{V}=\Omega_{\rm SP}(\hat{a}^\dagger+\hat{a})+\ \Omega_{\rm QE}(\hat{S}^++\hat{S}^-),\tag{4}$$

and expand the steady state wave-function in terms of the small parameter $E_{\rm L}$ as

$$|\psi\rangle=\sum_{n=0}E_{\rm L}^n|\psi_n\rangle,\tag{5}$$

where $|\psi_n\rangle$ belongs to the $n$-excitation manifold. As we are interested only in the scattering intensity and zero-delay second-order correlation function, the expansion above can be truncated at the two-excitation manifold. Once the perturbative solution to $\hat{H}_{\rm eff}|\psi\rangle=0$ is obtained, we can evaluate

$$I=\langle\psi_1|\hat{\mathbf{E}}_{\rm D}^-\hat{\mathbf{E}}_{\rm D}^+|\psi_1\rangle,\tag{6}$$

$$g^{(2)}(0)=\langle\psi_2|\hat{\mathbf{E}}_{\rm D}^-\hat{\mathbf{E}}_{\rm D}^-\hat{\mathbf{E}}_{\rm D}^+\hat{\mathbf{E}}_{\rm D}^+|\psi_2\rangle/I^2,\tag{7}$$

with $\hat{\mathbf{E}}_{\rm D}^-\propto\boldsymbol{\mu}_{\rm SP}\hat{a}^\dagger+\boldsymbol{\mu}_{\rm QE}\hat{S}^+$. Equations 6 and 7 lead to the analytical expressions in Equations (4) and (5) of the main text.

By construction, our approach yields exact results for low enough $E_{\rm L}$. This is shown in Figure 1 for the particular case of $N=5$ (same material parameters as in the main text). The upper (lower) panel shows intensity (photon correlations) versus laser frequency for five different values of the single-QE cooperativity, $C$. Color solid and black dotted lines plot full Liouvillian and effective Hamiltonian calculations, respectively. The former were obtained solving Equation (1) numerically and computing

$$I=\mathrm{Tr}\{\hat{\rho}\hat{\mathbf{E}}_{\rm D}^-\hat{\mathbf{E}}_{\rm D}^+\},\tag{8}$$

$$g^{(2)}(0)=\mathrm{Tr}\{\hat{\rho}\hat{\mathbf{E}}_{\rm D}^-\hat{\mathbf{E}}_{\rm D}^-\hat{\mathbf{E}}_{\rm D}^+\hat{\mathbf{E}}_{\rm D}^+\}/I^2.\tag{9}$$

The pumping parameters were set to $\Omega_{\rm SP}=19$ meV and $\Omega_{\rm QE}=1$ meV, and the steady-state density matrix was calculated up to the three-excitation manifold. In all cases, both solutions are in perfect agreement. Note that a rather moderate $N$ was chosen in the calculations to ensure the convergence of the Liouvillian calculations, which become cumbersome for larger ensemble sizes.

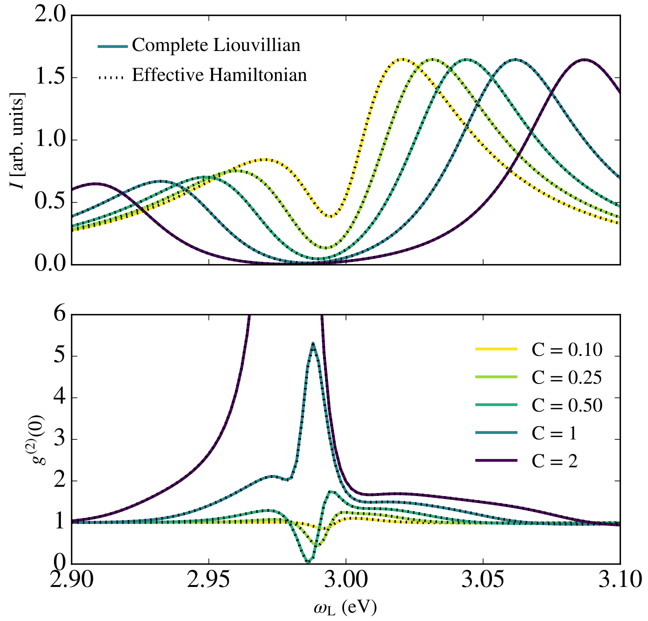


FIG. 1. Scattering intensity (top panel) and photon correlations (bottom panel) versus laser frequency for $N = 5$ QEs coupled to a SP cavity for various $C$. The excellent agreement between full Liouvillian (solid color lines) and effective Hamiltonian (black dotted lines) calculations prove the validity of the latter ($\Omega_{\rm SP} = 19$ meV, $\Omega_{\rm QE} = 1$ meV).

## SPATIAL INHOMOGENEITY OF THE PLASMON NEAR-FIELD

In this section, we analyze the effect that the introduction of spatial inhomogeneity in the SP near-field has on the scattering intensity and photon correlations for strongly coupled QE ensembles. A spatially dependent SP field, $\mathbf{E}_{\rm SP} = \mathbf{E}_{\rm SP}(\mathbf{r})$, leads to a coupling strength varying across the QE ensemble as

$$\lambda_i = \mathbf{E}_{\rm SP}(\mathbf{r}_i) \cdot \boldsymbol{\mu}_{{\rm QE},i} = E_{{\rm SP}\parallel}(\mathbf{r}_i)\mu_{\rm QE}, \qquad (10)$$

where $\mathbf{r}_i$ denotes the position of the $i$-th QE, and $E_{{\rm SP}\parallel}(\mathbf{r}_i)$ stands for the SP electric field component parallel to the QE dipole moment at this position. For simplicity, and as we are interested in exploring the spatial dependence of the plasmonic near-field, we assume that all the QE dipole moments are parallel and have the same magnitude.

Under low pumping conditions, the full Liouvillian describing the steady-state density matrix for a hybrid system, in which the QE-SP coupling is given by Equation (10), can still be mapped into an effective non-Hermitian Hamiltonian as in Equation (3). The Hamiltonian describing the coherent dynamics now has the form

$$\hat{H} = \Delta_{\rm SP}\hat{a}^\dagger\hat{a} + \Delta_{\rm QE}\hat{S}_z + \sum_{i=1}^{N}\lambda_i(\hat{\sigma}_i^\dagger\hat{a} + \hat{\sigma}_i\hat{a}^\dagger) + \\ +\Omega_{\rm SP}(\hat{a}^\dagger + \hat{a}) + \Omega_{\rm QE}(\hat{S}^+ + \hat{S}^-), \qquad (11)$$

where all the terms are defined in the main text. Note that the Lindblad terms can be still approximated in the form of Equations 1-3. Calculating the steady-state for Equation (11) requires accounting for not only the bright state of the QE ensemble but also all the dark states. This makes its computation much heavier, despite the fact that the perturbative treatment in Section 1 remains valid.

Figure 2 plots the scattering intensity (top panels) and zero-delay second-order correlation function (bottom panels) for QE-SP systems with five different single-emitter cooperativities. Dotted lines correspond to SP cavities with a uniform (homogeneous) electric near-field across the ensemble. Solid lines render $I$ and $g^{(2)}(0)$ for various degrees of spatial inhomogeneity in $E_{{\rm SP}\parallel}$: 20 (a), 50 (b) and 90% (c). Note that these percentages indicate the relative deviation of the extremal values of $\lambda_i$ [the rest of parameters remain as in Figure 3($b_1$)-($b_2$)]. In order to make a meaningful comparison between different systems, the collective coupling strength is kept constant in all cases (for a given single-emitter cooperativity), i.e.,

$$\sum_{i=1}^{N}\lambda_i^2 = N\gamma_{\rm SP}\gamma_{\rm QE}C/2. \qquad (12)$$

The top panels of Figure 2 demonstrate that the far-field intensity is very robust to variations in $\lambda_i$. In top panels (a) and (b), homogeneous and inhomogeneous calculations virtually overlap. Only at 90% plasmonic inhomogeneity, appreciable deviations between both sets of data take place. Note that the contrast between upper and lower PEP peaks decreases with spatial inhomogeneity. The bottom panels of Figure 2 show that photon correlations are more sensitive to $\mathbf{E}_{\rm SP}(\mathbf{r})$. We can observe that a non-uniform SP near-field leads to two main effects on $g^{(2)}(0)$. On the one hand, for high $C$, the bunching maxima broaden and their height increases. This removes regions of moderate antibunching that emerge for intermediate cooperativity ($C$=0.5) in the homogeneous case. On the other hand, at lower $C$, the deep antibunching minima shift towards higher $\omega_{\rm L}$, but the minimum in $g^{(2)}(0)$ presents a similar depth. In fact, the correlation minima at $C = 0.1$ and $C = 0.25$ are still slightly deeper in the inhomogeneous calculations. Despite these differences, Figure 2 proves that SP spatial inhomogeneities do not lead to qualitative changes in $I$ and $g^{(2)}(0)$.

## INHOMOGENEOUS BROADENING IN THE EMITTER ENSEMBLE

We study how inhomogeneous broadening of the QE transition frequencies affects the photon correlations in the hybrid QE-SP system. The Hamiltonian accounting for these effects has the form

$$\hat{H} = \Delta_{\rm SP}\hat{a}^\dagger\hat{a} + \sum_{i=1}^{N}\Delta_{{\rm QE},i}\hat{\sigma}_i^\dagger\hat{\sigma}_i + \lambda(\hat{S}^+\hat{a} + \hat{S}^-\hat{a}^\dagger) + \\ +\Omega_{\rm SP}(\hat{a}^\dagger + \hat{a}) + \Omega_{\rm QE}(\hat{S}^+ + \hat{S}^-), \qquad (13)$$

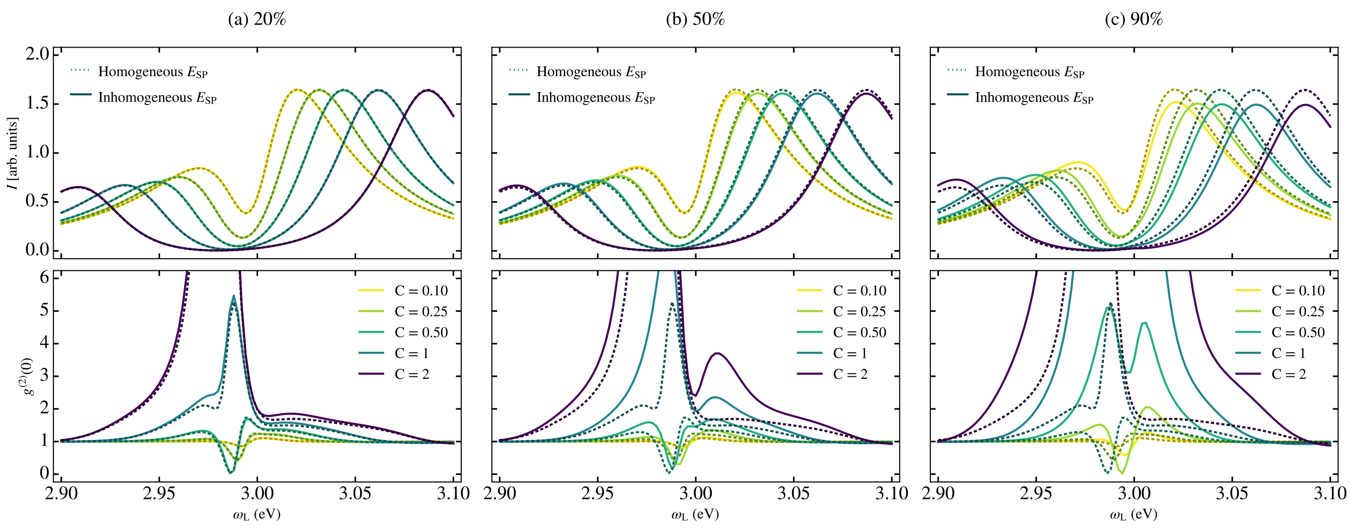


FIG. 2. Scattering intensity $I$ (top) and zero-delay second-order correlation function $g^{(2)}(0)$ (bottom) versus laser frequency for various $C$-values. Solid lines correspond to spatially inhomogeneous SP near-fields with 20 (a), 50 (b) and 90% (c) variation in $E_{\mathrm{SP}\parallel}$ within the QE ensemble. Dotted lines (the same in all cases) render homogeneous (uniform $E_{\mathrm{SP}\parallel}$) results.

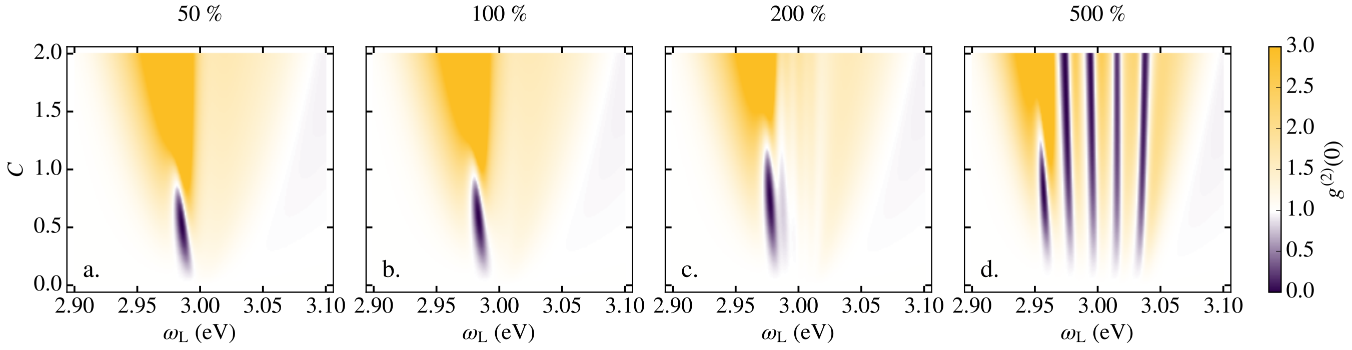


FIG. 3. Second-order correlation function versus $\omega_{\mathrm{L}}$ and $C$ for a QE ensembles with $\gamma_{\mathrm{QE}}^{\mathrm{nr}} = 15$ meV. The QE transition frequencies are uniformly distributed around $\omega_{\mathrm{SP}}$. The percentages indicate the extremal values of the ratio $|\omega_{\mathrm{QE},i} - \omega_{\mathrm{SP}}|/\gamma_{\mathrm{QE}}^{\mathrm{nr}}$ in each panel.

where $\Delta_{\mathrm{QE},i} = \omega_{\mathrm{QE},i} - \omega_{\mathrm{L}}$ and $\omega_{\mathrm{QE},i}$ is the transition frequency for the $i$-th QE. The description of radiative and nonradiative damping remains the same as in Equation (2). Like in the previous section, obtaining the steady-state for the Hamiltonian in Equation (13) requires considering the dark states of the QE ensemble, even in its perturbative treatment.

Figure 3 displays $g^{(2)}(0)$ versus laser frequency and cooperativity $C$ for inhomogeneously broaden QE ensembles ($N = 5$). All the parameters remain the same as in Figure 3(b$_1$)-(b$_2$), except for the QE transition frequencies, which are now uniformly distributed around $\omega_{\mathrm{SP}} = 3$ eV. The minimum and maximum values of the ratio $|\omega_{\mathrm{QE},i} - \omega_{\mathrm{SP}}|/\gamma_{\mathrm{QE}}^{\mathrm{nr}}$ are indicated by the percentages above each panel. Panels (a) and (b) show that photon correlations are not affected by differences in the emission frequencies if these are smaller than or comparable to $\gamma_{\mathrm{QE}}^{\mathrm{nr}} = 15$ meV. In panel (c), the spectral broadening is twice larger than the nonradiative decay rate, and we can observe that the region of antibunching is slightly distorted and extents into larger $C$ values. Finally, five well defined spectral lines (as many as QEs in the ensemble) yielding $g^{(2)}(0) < 1$ are apparent in panel (d). In this case, $|\omega_{\mathrm{QE},i} - \omega_{\mathrm{SP}}|$ is up to five times larger than $\gamma_{\mathrm{QE}}^{\mathrm{nr}}$ and the photon correlation maps are qualitatively different from those obtained for identical QEs. Thus, Figure 3 shows that a large QE nonradiative decay rate (low quantum yield) increases the robustness of the hybrid system against inhomogeneous broadening effects.

## EFFECT OF PLASMON LOSSES AND EMITTER NONRADIATIVE DECAY

We investigate now the effect of SP damping and QE nonradiative decay on the correlations of the photon scattered by hybrid QE-SP systems. Here, we neglect spectral inho-

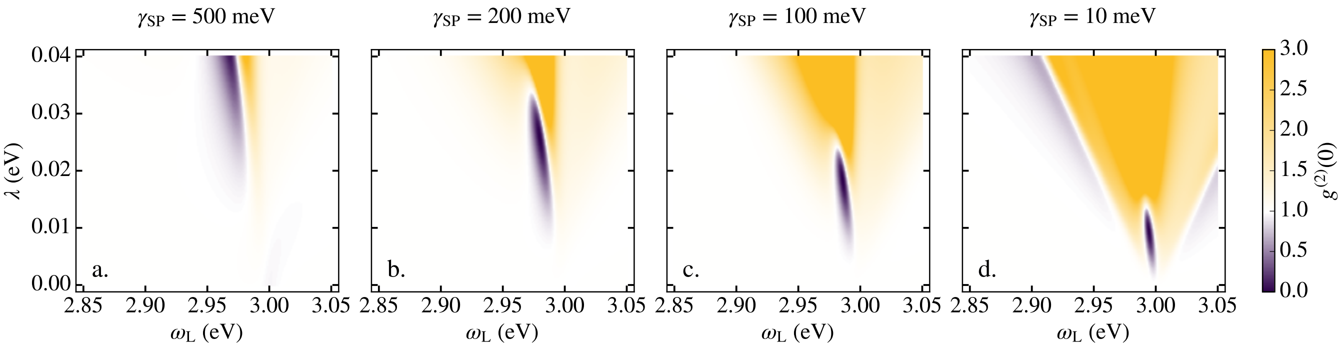


FIG. 4. Zero-delay second-order correlation function versus laser frequency and coupling strength, $\lambda$, for QE ensembles coupled to SP cavities with four different SP decay rates $\gamma_{SP}$.

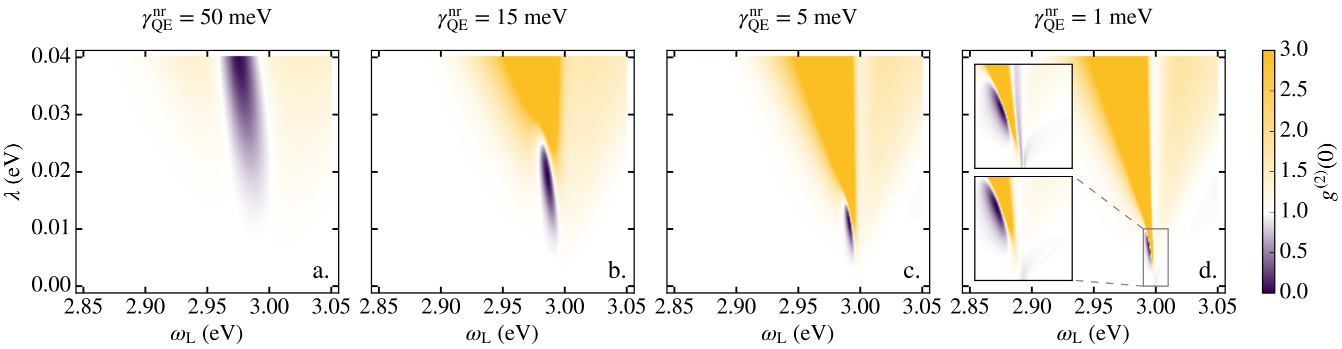


FIG. 5. Zero-delay second-order correlation function versus laser frequency and coupling strength, $\lambda$, for QE ensembles coupled to SP cavities with four different QE nonradiative decay rates $\gamma_{QE}^{nr}$.

mogeneities in the ensemble, and focus on emitters with identical $\omega_{QE}$ and $\gamma_{QE}^{nr}$.

Figure 4 displays photon correlation maps for values of the SP damping rate ranging from 500 meV to 10 meV. In order to allow the comparison between different systems, the coupling strength is expressed in terms of $\lambda$, instead of the single-emitter cooperativity. Panel (c) corresponds to the case considered in the main text [see Figure 3($b_2$)]. Panels (a) and (b) show that the regions yielding strong photon correlations widen significantly (both in $\lambda$ and $\omega_L$) by increasing $\gamma_{SP}$. This broadening is accompanied by a slight shift towards higher coupling strengths. On the contrary, bunching and antibunching take place at sharper spectral windows and smaller $\lambda$ for lower SP damping, see panel (d). The comparison against panel (c) indicates that the asymmetry in $g^{(2)}(0)$ around the resonant condition $\omega_L = \omega_{QE-SP}$ diminishes with decreasing $\gamma_{SP}$. More interestingly, for larger $\lambda$, the system develops a rather spectrally symmetric correlation function maximum (strong bunching) centered at $\omega_{QE-SP}$. This is accompanied by two $g^{(2)}(0)$ minimum side bands. Thus, Figure 4(d) reproduces the so-called photon tunnelling and blockade phenomenology recently reported for single quantum dots strongly coupled to semiconductor microcavities under coherent pumping [3, 4].

Figure 5 renders $g^{(2)}(0)$ as a function of the laser frequency and coupling strength for identical QEs with different $\gamma_{QE}^{nr}$. Panel (b), which reproduces Figure 3($b_2$) and corresponds to QEs with very low quantum yield ($7 \cdot 10^{-5}$), is taken as reference. By increasing $\gamma_{QE}^{nr}$, the region of antibunching widens in $\omega_L$ and moves to higher values of the cooperativity, see panel (a). On the contrary, panel (c) shows that by reducing the QE nonradiative decay rate, $g^{(2)}(0) < 1$ takes place into narrower spectral windows at lower $C$. As expected, this phenomenology is very similar to the one shown in Figure 4, as both QE and SP plasmon decay contribute in the same way to the PEP linewidth. Panel (d) displays photon correlations for QEs with a quantum yield of $10^{-3}$, showing the same trend as panels (a)-(c). The bottom inset zooms into the antibunching region. The top inset renders $g^{(2)}(0)$ within the same window but for emitters with a quantum yield of 0.5 ($\gamma_{QE}^{nr} = \gamma_{QE}^{r} = 6\mu$eV). Only within this region, the correlation functions for both systems present a slight difference. Note that the latter develops an extremely narrow and rather shallow antibunching band close to the condition $\omega_L = \omega_{QE,SP}$.

The parametric studies presented in Figure 4 and Figure 5 show that the significant nonradiative losses inherent to organic molecules and plasmonic cavities allow for the

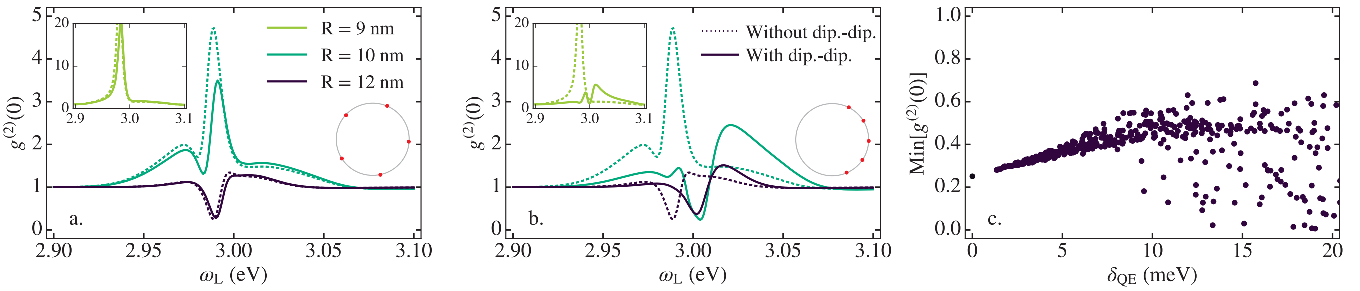


FIG. 6. (a,b) Zero-delay second-order correlation function versus laser frequency for 5 QEs evenly distributed along 3 rings of different radii $R$. In (a), the ensembles are evenly spread along the whole ring perimeter ($2\pi$ radians), whereas in (b), the QE ensemble ranges only over an arc of $0.88\pi$ radians. In all cases, solid (dotted) lines correspond to interacting (non-interacting) QEs. (c) The minimum value of $g^{(2)}(0)$ for a large number of random distributions of emitters on the ring with $R = 12$ nm, plotted as a function of $\delta_{\text{QE}}$, the maximum energy shift induced by QE-QE interactions.

generation of robust photon correlations in PEP systems.

## IMPACT OF EMITTER-EMITTER INTERACTIONS

Finally, we explore how photon correlations are altered when dipole-dipole interactions within the emitter ensemble are taken into account. These are described by adding new terms to $\hat{H}$ given in Equation (2) of the main text. The new Hamiltonian now acquires the form

$$\hat{H}' = \hat{H} + \frac{1}{2}\sum_{i\neq j} V_{ij}[\hat{\sigma}_i^\dagger\hat{\sigma}_j + \hat{\sigma}_j^\dagger\hat{\sigma}_i], \qquad (14)$$

where indices $i$ and $j$ run from 1 to $N$. The implementation of Equation (14) requires considering a specific configuration of the PEP system. In the following, and for simplicity, we assume that all QEs are placed along a ring of radius $R$, and that their dipole moments are all parallel and normal to the ring plane. In this configuration, the interaction strength is given by [5]

$$V_{ij} = \frac{\mu_{\text{QE}}^2}{4\pi\epsilon_0|\mathbf{r}_i - \mathbf{r}_j|^3} \qquad (15)$$

with $|\mathbf{r}_i - \mathbf{r}_j| \propto R$. Note that all QEs are identical and are coupled with the same strength, $\lambda$, to the SP cavity. Previous theoretical studies on single-particle and dimer nanocavities [6, 7] have shown that $\lambda$ scales with the volume of the system, in a similar way as Equation (15). Therefore, increasing the radius of the QE distribution does not alter the ratio $V_{ij}/\lambda$.

Figure 6 plots $g^{(2)}(0)$ versus laser frequency for 5-QE ensembles distributed for $R = 9$, 10, and 12 nm. We model the nanocavity as a silver nanosphere with radius of 6 nm in the center of the QE ring. Using Ref. 6, we compute the coupling strength for the dipolar SP mode supported by the system, obtaining $\lambda = 37$, 27, and 16 meV for $R = 9$, 10, and 12 nm, respectively. In the left and central panels of Figure 6, dotted lines render $g^{(2)}(0)$ obtained within the non-interacting QE approximation. These spectra correspond to cuts at single-emitter cooperativities, $C$, equal to 1.80 (green), 0.98 (blue) and 0.35 (violet) in Figure 3($b_2$) in the main text. The three $R$'s have been chosen so that the smallest yields a broad bunching maxima and the largest a narrow antibunching dip, with an intermediate configuration in between.

Solid lines in the left panel of Figure 6 plot $g^{(2)}(0)$ for interacting QEs evenly distributed along the ring ($2\pi$ radians). We can observe that the impact of dipole-dipole interactions in photon correlations is moderate for the three QE ensembles, with the smallest effect in the antibunching case ($R = 12$ nm). As the ratio $V_{ij}/\lambda$ is the same for all $R$, we can infer that there is another energy scale that affects the sensitivity of the system to QE interactions. Solid lines in the central panel of Figure 6 show photon correlation spectra for an ensemble that spreads only within $0.88\pi$ radians along the ring (see insets). By varying the angular extent of the QE arrangement, all the parameters except for $V_{ij}$ remain the same as in the left panel. Specifically, the nearest-neighbour interaction strength is enhanced by a factor 9.7 for all ring radii, leading to a more significant impact of dipole-dipole interactions on $g^{(2)}(0)$. Interestingly, we again find that while bunching (observed at $R = 9$ and 10 nm) is severely impacted by interactions, the antibunching observed at $R = 12$ nm is quite robust, with $g^{(2)}(0)$ showing almost the same shape but shifted in energy compared to the non-interacting case. In order to explore this in more detail, the right panel of Figure 6 shows the minimum value of $g^{(2)}(0)$ obtained for a large number of completely random configurations of emitters along the ring, plotted as a function of $\delta_{\text{QE}}$, the largest energy shift obtained by diagonalizing just the emitter-emitter interaction. This shows that the degree of antibunching in the system is quite robust against emitter-emitter interactions and only slowly decreases as the interaction-induced shifts increase. Once the interactions become comparable to the emitter linewidth $\gamma_{\text{QE}} = 15$ meV, a similar regime as under large inhomogeneous broadening is entered (see Figure 3). The plasmon then does not couple collectively to all emitters, but almost

independently to different energetically resolved superpositions of emitters. This leads to an effective interaction with fewer QEs, and thus even more pronounced antibunching in some cases.

* a.fernandez-dominguez@uam.es
† fj.garcia@uam.es

[1] P. M. Visser and G. Nienhuis, "Solution of quantum master equations in terms of a non-Hermitian Hamiltonian," Phys. Rev. A **52**, 4727-4736 (1995).

[2] R. J. Brecha, P. R. Rice, and M. Xiao, "N two-level atoms in a driven optical cavity: quantum dynamics of forward photon scattering for weak incident fields," Phys. Rev. A **59**, 2392-2417 (1999).

[3] K. Müller, A. Rundquist, K. A. Fisher, T. Sarmiento, K. G. Lagoudakis, Y. A. Kelaita, C. Sánchez-Muñoz, E. del Valle, F. P. Laussy, and J. Vučković, "Coherent generation of nonclassical light on chip via detuned photon blockade," Phys. Rev. Lett. **114**, 233601 (2015).

[4] A. Faraon, I. Fushman, D. Englund, N. Stoltz, P. Petroff, and J. Vučković, "Coherent generation of non-classical light on a chip via photon-induced tunnelling and blockade," Nat. Phys. **8**, 859-863 (2008).

[5] J. Feist and F. J. García-Vidal, "Extraordinary exciton conductance induced by strong coupling," Phys. Rev. Lett. **114**, 196402 (2015).

[6] A. Delga, J. Feist, J. Bravo-Abad, and F. J. García-Vidal, "Quantum emitters near a metal nanoparticle: strong coupling and quenching," Phys. Rev. Lett. **112**, 253601 (2014).

[7] R.-Q. Li, D. Hernangómez-Pérez, F. J. García-Vidal, and A. I. Fernández-Domínguez, "Transformation optics approach to plasmon-exciton strong coupling in nanocavities," Phys. Rev. Lett. **117**, 107401 (2016).
